# Supplementary material for: Massive Spikes in LLMs are Bias Vectors: Mechanistic Uncovering and Spike-Free Quantization
Source: arXiv:2606.02288 source file (2026-06-01)
Supplement: Supplementary file 1 [file complete_results.tex]

\section{Complete Results for Main Result Table}
\label{app:complete_result}
The complete results are shown in Table \ref{tab:full_result}.
\begin{table*}[t]
\centering
\scriptsize 
 
\setlength{\tabcolsep}{2.5pt}

\caption{\textbf{Detailed results for LLM quantization.} We report per-task accuracy on common-sense reasoning benchmarks: \textit{acc} for BoolQ, SIQA, and WinoGrande, and \textit{acc\_norm} for ARC-e, ARC-c, PIQA, HellaSwag, and OBQA. \textbf{Avg. Acc.} denotes the mean across tasks. We also report WikiText2 perplexity at context lengths 2048 and 8192 (lower is better). ``d'' and ``s'' indicate per-token dynamic and per-tensor static activation quantization, respectively. All methods are evaluated without fine-tuning and use the same calibration setting. LLaMA2-7b does not natively support 8192 sequence lengths and is excluded from those evaluations.}
\label{tab:full_result}

\begin{tabular}{c|cc|ccccccccc|cc}
\hline
\textbf{Model} & \textbf{Bits} & \textbf{Method} & \textbf{ARC-e} & \textbf{ARC-c} & \textbf{BoolQ} & \textbf{PIQA} & \textbf{SIQA} & \textbf{HellaS.} & \textbf{OBQA} & \textbf{WinoG.} & \textbf{Avg. Acc.} & \textbf{Wiki} & \textbf{Wiki} \\
 & W-A-KV & & & & & & & & & & & \textbf{(2048)} & \textbf{(8192)} \\ \hline

% =========================================================
% MODEL 1: Llama-2-7B
% =========================================================
\multirow{19}{*}{Llama-2-7B} & 16-16-16 & Baseline & 73.78 & 44.97 & 79.33 & 78.67 & 32.91 & 76.15 & 44.00 & 69.38 & 62.40 & 5.47 & - \\ \cdashline{2-14}
 & \multirow{4}{*}{4-8d-8} & RTN & 71.80 & 44.28 & 76.27 & 78.02 & 32.80 & 74.55 & 42.00 & 68.35 & 61.01 & 5.88 & - \\
 & & QuaRot-RTN & 44.23 & 26.28 & 56.79 & 64.15 & 33.73 & 41.66 & 29.40 & 54.46 & 43.84 & 30.19 & - \\
 & & PrefixQuant & 73.99 & 43.86 & 77.74 & 78.07 & 33.01 & 75.33 & 43.00 & 69.69 & 61.84 & 5.66 & - \\
 & & InsertQuant & 72.98 & 43.34 & 77.77 & 79.05 & 32.96 & 74.77 & 43.00 & 68.75 & 61.58 & 5.68 & - \\ \cdashline{2-14}
 & \multirow{4}{*}{4-8d-4} & RTN & 70.37 & 43.09 & 75.02 & 78.24 & 33.01 & 73.56 & 41.00 & 67.48 & 60.22 & 6.04 & - \\
 & & QuaRot-RTN & 44.23 & 26.28 & 56.79 & 64.15 & 33.73 & 41.66 & 29.40 & 54.46 & 43.84 & 30.19 & - \\
 & & PrefixQuant & 72.98 & 43.94 & 77.83 & 77.86 & 33.11 & 75.24 & 43.40 & 68.27 & 61.58 & 5.70 & - \\
 & & InsertQuant & 73.19 & 42.83 & 77.03 & 78.89 & 33.21 & 74.47 & 43.40 & 68.67 & 61.46 & 5.73 & - \\ \cdashline{2-14}
 & \multirow{3}{*}{4-8s-4} & RTN & 39.18 & 27.73 & 56.09 & 60.17 & 33.16 & 43.11 & 28.00 & 53.75 & 42.65 & 30.84 & - \\
 & & PrefixQuant & 72.94 & 43.09 & 77.71 & 77.86 & 32.75 & 74.87 & 42.60 & 68.75 & 61.32 & 5.77 & - \\
 & & InsertQuant & 72.90 & 42.58 & 77.19 & 78.35 & 33.11 & 73.97 & 43.20 & 68.27 & 61.19 & 5.84 & - \\ \cdashline{2-14}
 & \multirow{4}{*}{4-4d-4} & RTN & 27.90 & 24.57 & 56.21 & 53.21 & 33.67 & 29.97 & 26.60 & 49.33 & 37.68 & 439 & - \\
 & & QuaRot-RTN & 34.97 & 23.29 & 58.23 & 59.14 & 32.50 & 36.73 & 27.00 & 51.22 & 40.39 & 45.69 & - \\
 & & PrefixQuant & 70.24 & 43.17 & 74.59 & 75.73 & 33.47 & 74.38 & 42.80 & 66.85 & 60.15 & 6.27 & - \\
 & & InsertQuant & 69.74 & 42.83 & 73.58 & 76.99 & 33.11 & 72.92 & 41.00 & 66.14 & 59.54 & 6.30 & - \\ \cdashline{2-14}
 & \multirow{3}{*}{4-4s-4} & RTN & 26.22 & 28.41 & 43.76 & 48.37 & 32.29 & 25.43 & 26.40 & 48.15 & 34.88 & 7072 & - \\
 & & PrefixQuant & 71.38 & 42.83 & 75.96 & 77.69 & 32.75 & 73.57 & 40.60 & 67.72 & 60.31 & 6.22 & - \\
 & & InsertQuant & 70.20 & 43.17 & 74.92 & 77.09 & 33.01 & 72.38 & 41.20 & 65.19 & 59.65 & 6.30 & - \\ \hline

% =========================================================
% MODEL 2: Llama-3-8B
% =========================================================
\multirow{19}{*}{Llama-3-8B} & 16-16-16 & Baseline & 77.53 & 54.10 & 82.26 & 80.63 & 33.01 & 79.24 & 44.80 & 73.80 & 65.67 & 6.14 & 5.54 \\ \cdashline{2-14}
 & \multirow{4}{*}{4-8d-8} & RTN & 74.49 & 47.10 & 80.24 & 78.02 & 32.91 & 77.22 & 46.00 & 72.14 & 63.51 & 7.58 & 6.89 \\
 & & QuaRot-RTN & 69.02 & 42.75 & 66.76 & 74.59 & 33.27 & 69.97 & 40.00 & 70.88 & 58.40 & 9.45 & 8.32 \\
 & & PrefixQuant & 76.81 & 52.65 & 80.40 & 79.11 & 32.96 & 77.91 & 43.80 & 72.61 & 64.53 & 6.81 & 6.14 \\
 & & InsertQuant & 76.94 & 52.22 & 80.46 & 79.71 & 33.32 & 78.17 & 43.20 & 71.90 & 64.49 & 6.83 & 6.14 \\ \cdashline{2-14}
 & \multirow{4}{*}{4-8d-4} & RTN & 74.03 & 46.76 & 73.64 & 75.90 & 32.91 & 75.89 & 43.40 & 70.64 & 61.65 & 8.08 & 7.39 \\
 & & QuaRot-RTN & 69.02 & 42.75 & 66.76 & 74.59 & 33.27 & 69.97 & 40.00 & 70.88 & 58.40 & 9.45 & 8.32 \\
 & & PrefixQuant & 75.63 & 52.82 & 79.63 & 79.54 & 32.91 & 77.75 & 43.00 & 70.72 & 64.00 & 6.91 & 6.23 \\
 & & InsertQuant & 75.76 & 51.02 & 80.64 & 79.11 & 33.01 & 77.53 & 43.60 & 72.45 & 64.14 & 6.92 & 6.23 \\ \cdashline{2-14}
 & \multirow{3}{*}{4-8s-4} & RTN & 42.93 & 26.11 & 55.44 & 62.02 & 32.55 & 42.49 & 29.80 & 53.75 & 43.14 & 64.25 & 61.09 \\
 & & PrefixQuant & 75.93 & 51.62 & 79.88 & 78.89 & 32.96 & 77.28 & 42.80 & 71.67 & 63.88 & 7.00 & 6.31 \\
 & & InsertQuant & 74.79 & 50.09 & 78.96 & 78.73 & 33.01 & 77.28 & 45.20 & 71.43 & 63.68 & 7.07 & 6.38 \\ \cdashline{2-14}
 & \multirow{4}{*}{4-4d-4} & RTN & 37.37 & 25.00 & 50.55 & 56.80 & 32.50 & 37.84 & 29.80 & 49.01 & 39.86 & 167.37 & 189 \\
 & & QuaRot-RTN & 57.28 & 32.08 & 58.10 & 66.27 & 32.80 & 58.52 & 35.40 & 58.01 & 49.81 & 17.91 & 14.88 \\
 & & PrefixQuant & 70.37 & 46.16 & 74.19 & 76.55 & 32.70 & 75.17 & 38.60 & 66.85 & 60.07 & 8.13 & 7.30 \\
 & & InsertQuant & 71.09 & 45.05 & 71.28 & 75.35 & 32.86 & 75.57 & 41.60 & 65.98 & 59.85 & 8.19 & 7.34 \\ \cdashline{2-14}
 & \multirow{3}{*}{4-4s-4} & RTN & 25.34 & 23.98 & 39.30 & 51.36 & 31.88 & 26.38 & 25.00 & 53.04 & 34.53 & 5647 & 4970 \\
 & & PrefixQuant & 72.94 & 45.39 & 76.27 & 77.64 & 33.11 & 75.23 & 41.40 & 67.64 & 61.20 & 8.35 & 7.51 \\
 & & InsertQuant & 72.31 & 46.59 & 69.14 & 75.90 & 32.55 & 74.20 & 39.60 & 65.75 & 59.50 & 8.91 & 8.12 \\ \hline

% =========================================================
% MODEL 3: Mistral-7B
% =========================================================
\multirow{19}{*}{Mistral-7B} & 16-16-16 & Baseline & 80.05 & 54.35 & 83.70 & 81.99 & 32.91 & 80.69 & 47.20 & 74.03 & 66.87 & 5.32 & 4.75 \\ \cdashline{2-14}
 & \multirow{4}{*}{4-8d-8} & RTN & 79.04 & 51.54 & 82.08 & 80.52 & 32.91 & 79.27 & 46.80 & 72.69 & 65.61 & 6.48 & 5.17 \\
 & & QuaRot-RTN & 68.06 & 42.83 & 79.91 & 77.58 & 32.91 & 75.08 & 41.00 & 71.03 & 61.05 & 6.75 & 5.94 \\
 & & PrefixQuant & 78.96 & 52.73 & 82.48 & 80.85 & 32.91 & 79.98 & 44.00 & 72.38 & 65.53 & 5.52 & 4.91 \\
 & & InsertQuant & 76.81 & 49.91 & 83.82 & 80.96 & 32.91 & 77.41 & 45.40 & 72.93 & 65.02 & 5.72 & 5.04 \\ \cdashline{2-14}
 & \multirow{4}{*}{4-8d-4} & RTN & 78.79 & 50.60 & 82.35 & 80.85 & 32.91 & 78.56 & 45.80 & 71.82 & 65.21 & 6.45 & 5.42 \\
 & & QuaRot-RTN & 68.06 & 42.83 & 79.91 & 77.58 & 32.91 & 75.08 & 41.00 & 71.03 & 61.05 & 6.75 & 5.94 \\
 & & PrefixQuant & 79.08 & 52.13 & 82.81 & 80.79 & 32.91 & 79.91 & 43.80 & 71.82 & 65.41 & 5.56 & 4.95 \\
 & & InsertQuant & 75.88 & 49.15 & 83.82 & 80.85 & 32.96 & 77.12 & 44.80 & 72.14 & 64.59 & 5.76 & 5.10 \\ \cdashline{2-14}
 & \multirow{3}{*}{4-8s-4} & RTN & 49.37 & 27.90 & 50.18 & 60.39 & 32.09 & 36.20 & 29.60 & 54.30 & 42.50 & 243 & 612 \\
 & & PrefixQuant & 78.28 & 51.37 & 82.60 & 80.41 & 32.91 & 79.71 & 43.80 & 72.45 & 65.19 & 5.60 & 4.99 \\
 & & InsertQuant & 75.93 & 48.81 & 82.94 & 81.07 & 32.86 & 76.87 & 44.40 & 72.38 & 64.40 & 5.79 & 5.14 \\ \cdashline{2-14}
 & \multirow{4}{*}{4-4d-4} & RTN & 45.33 & 28.16 & 52.29 & 59.25 & 32.45 & 40.71 & 27.00 & 50.51 & 41.96 & 356 & 16.48 \\
 & & QuaRot-RTN & 63.59 & 38.65 & 74.50 & 74.27 & 32.80 & 68.59 & 39.40 & 63.77 & 56.95 & 8.10 & 6.93 \\
 & & PrefixQuant & 76.68 & 48.63 & 78.93 & 79.82 & 32.91 & 78.58 & 42.80 & 68.43 & 63.35 & 5.90 & 5.25 \\
 & & InsertQuant & 72.94 & 47.78 & 79.88 & 78.67 & 32.96 & 74.26 & 42.20 & 68.43 & 62.14 & 6.24 & 5.51 \\ \cdashline{2-14}
 & \multirow{3}{*}{4-4s-4} & RTN & 26.22 & 29.10 & 40.89 & 49.46 & 31.83 & 26.13 & 23.80 & 48.86 & 34.53 & INF & INF \\
 & & PrefixQuant & 77.53 & 49.49 & 82.08 & 79.27 & 32.86 & 78.89 & 43.20 & 70.17 & 64.18 & 5.90 & 5.26 \\
 & & InsertQuant & 73.27 & 47.78 & 81.77 & 79.16 & 32.96 & 74.94 & 44.00 & 70.72 & 63.08 & 6.14 & 5.50 \\ \hline

\end{tabular}
\end{table*}
